# Supplementary material for: Dataflow programming for the analysis of molecular dynamics with AViS, an analysis and visualization software application
Source: arXiv:1911.08882 ancillary file (2019-11-19)
Supplement: Supplementary file 1 [file suppl.pdf]

# Dataflow Programming for the Analysis of Molecular Dynamics with AViS, an Analysis and Visualization Software Application

**Kai Pua**[1,†], **Daisuke Yuhara**[1], **Sho Ayuba**[1], **Kenji Yasuoka**[1,*]

[1]Department of Mechanical Engineering, Keio University, 3-14-1 Hiyoshi, Kohoku-ku, Yokohama, Kanagawa, Japan 223-8522
[†]Current Address: Department of Computer Science, Graduate School of Information Science and Technology, University of Tokyo, 7-3-1 Hongo, Bunkyo-ku, Tokyo, JAPAN 113-8656
[*]yasuoka@mech.keio.ac.jp

## Supplementary Materials

**S1 Table.** Examples of in-built nodes provided by AViS. Custom nodes can be implemented by the user to interact with internal nodes, regardless of language.

| | |
|---|---|
| Particle Data | coordinates and trajectories of all atoms |
| System Info | configuration information of the loaded system |
| Get / Set Attribute | Read / Write per-atom attribute data |
| Set Radius Scale | Scale the radius of atoms |
| Show Range | Show / Hide atoms based on unique values |
| Add Bonds | Draw additional atom-atom bonds |
| Draw Surface | Draw an equi-value 3D surface |
| To Adjacency / Paired List | Converts the data storage format for connectivity lists |
| Plot Data | Plots a graph of arbitrary data |

**S1 Appendix.** a valid fortran analysis script that generates a sine wave

```
module makesin
    use iso_c_binding
    implicit none
!@in
    integer :: count = 0
!@in
    real*8 :: scale = 0
!@out
    real*8, allocatable, target :: result(:)
    contains
!@entry
    subroutine execute()
        integer :: a
        if (allocated(result)) deallocate(result)
        allocate(result(1:count))
        do a = 1, count
            result(a) = sin(a*scale)
        end do
    end subroutine execute
end module makesin
```

**S2 Appendix.** A valid Python analysis script that differentiates an array

```
import numpy as np

#@in list(1d)
arr = np.zeros(1)
#@out list(1d)
res = np.zeros(1)

#@entry
def Do():
    global arr, res
    res = np.diff(arr)
```

**S3 Appendix.** A valid C++ analysis script that applies an exponential decay to a signal

```
#include <cmath>

//@in cnt
double* array = 0;
//@in
double mag = 0;
//@out cnt
double* out = 0;
//@var
int cnt = 0;

//@entry
void execute() {
    if (out) delete[](out);
    out = new double[cnt];
    for (int a = 0; a < cnt; a++) {
        out[a] = array[a] * std::exp(-a * mag);
    }
}
```

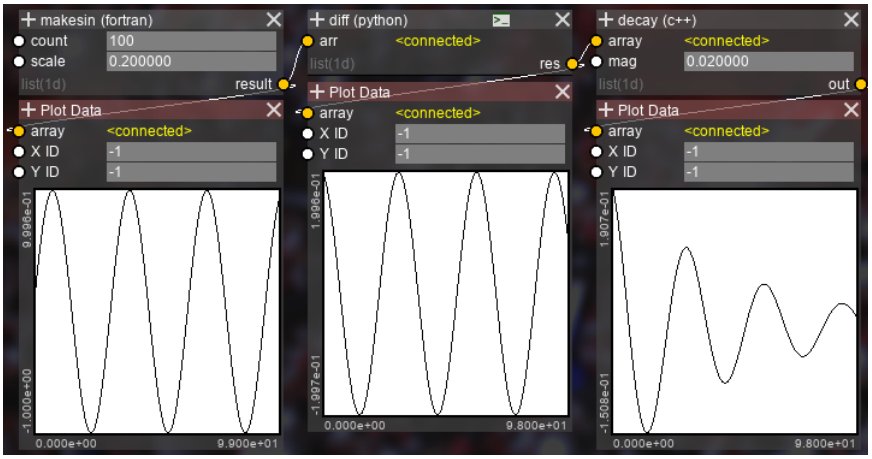


**S1 Fig..** Multi-language support for analysis. AViS handles data transfer between Fortran, Python, and C++ scripts automatically, including arrays as seen here.

**S4 Appendix.** Comment syntax for Fortran scripts

```
!all comments start with '!@'
!input variables are declared with 'in'
!output variables are declared with 'out'
!supported types are integer*2, integer, real*8

!a scalar variable
!@in
integer*2 :: foo = 0
!@in
integer :: bar = 0

!an array variable is an allocatable
!@out
real*8, allocatable, target :: baz (:,:)

!the function to be executed is declared with 'entry'
!@entry
subroutine exec()
```

**S5 Appendix.** Comment syntax for Python scripts

```
#arrays are declared with numpy
import numpy as np

#all comments start with '#@'
#input variables are declared with 'in'
#output variables are declared with 'out'
#the type of variable must be specified after the declaration

#a scalar variable
#supported types: short, int, double
#@in int
foo = 0
#@out double
bar = 1.0

#an array variable is a numpy ndarray
#type is 'list(nt)' where n=dimension and t=first character of the type (s, i, d)
#@out list(1d)
baz = numpy.ones(5)
#@out list(2s)
qux = numpy.zeros((1, 1), dtype=np.int16)

#the function to be executed is declared with 'entry'
#@entry
def Exec():
```

**S6 Appendix.** Comment syntax for C++ scripts

```
//all comments start with '//@'
//input variables are declared with 'in'
//output variables are declared with 'out'

//a scalar variable
//supported types are short, int, double
//@in
int foo = 0;
//@out
double bar = 1.0;

//an array variable is a pointer
//for each dimension, an int variable holding the size must be specified
//a 2-dimensional array, the element at (a, b) is [ny * a + b]
//@out nx, ny
double* baz = new double[4];

//for each variable used as the array size holder,
//if the variable is not used as input or output,
//it must be declared with 'var'
//@out
int nx = 2;
//@var
int ny = 2;

//the function to be executed is declared with 'entry'
//@entry
void Exec() {
```

**S7 Appendix.** An example of a SSV file with rotational and potential attributes. Each entry in the first line represents the type of data in each column.

```
# posx posy posz attr=rotx attr=roty attr=rotz attr=potential
1000
    0.0  1.0  0.5  0.0      1.0      0.0      −0.1
    0.2  0.8  0.3  1.0      0.0      0.0      −0.2
...
```

(a)

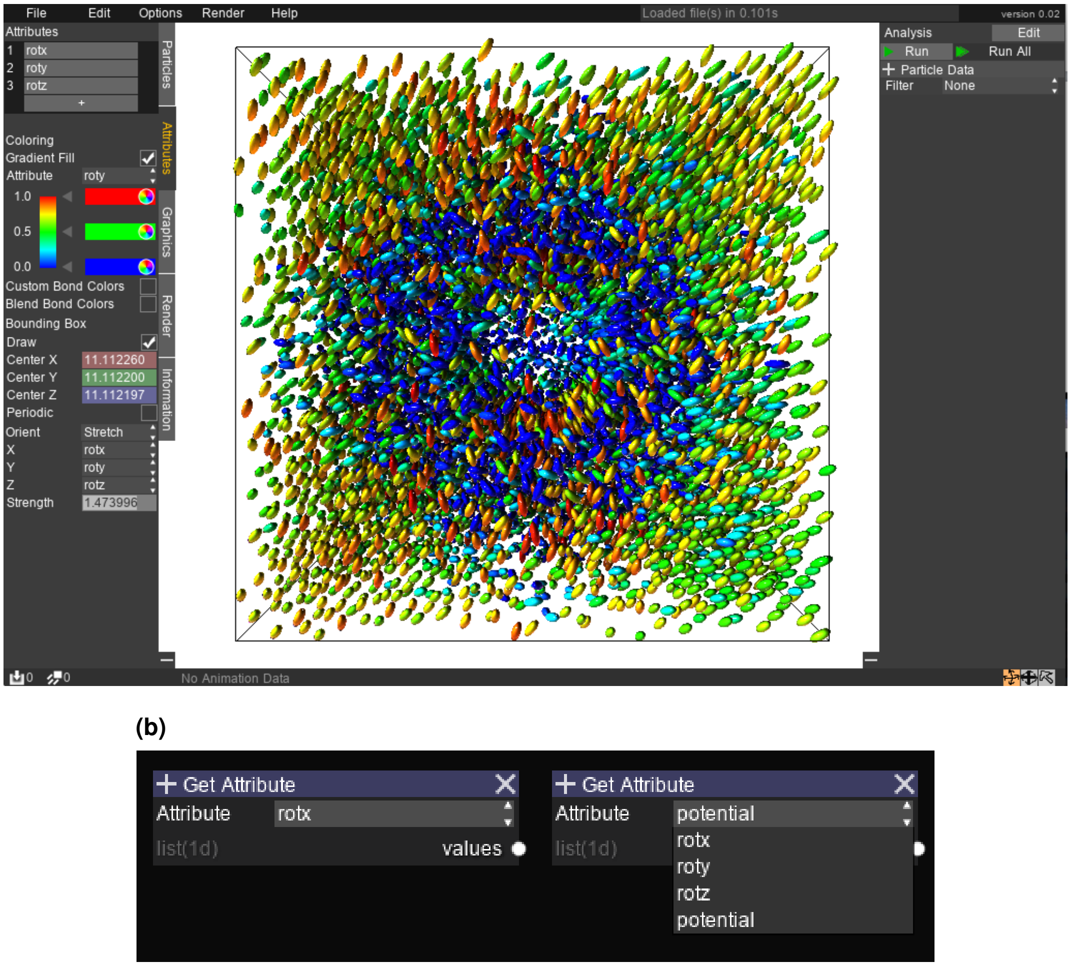


**S2 Fig..** Visualization and analysis of molecules with attribute data. (a) By importing the orientation data as attributes with the Generic SSV format, liquid crystal molecules can be visualized without the need to write a custom plugin or importer. In this figure, a color gradient is also applied based on the *roty* attribute. (b) Individual attributes can be used in analysis by utilizing the *Get Attribute* node.

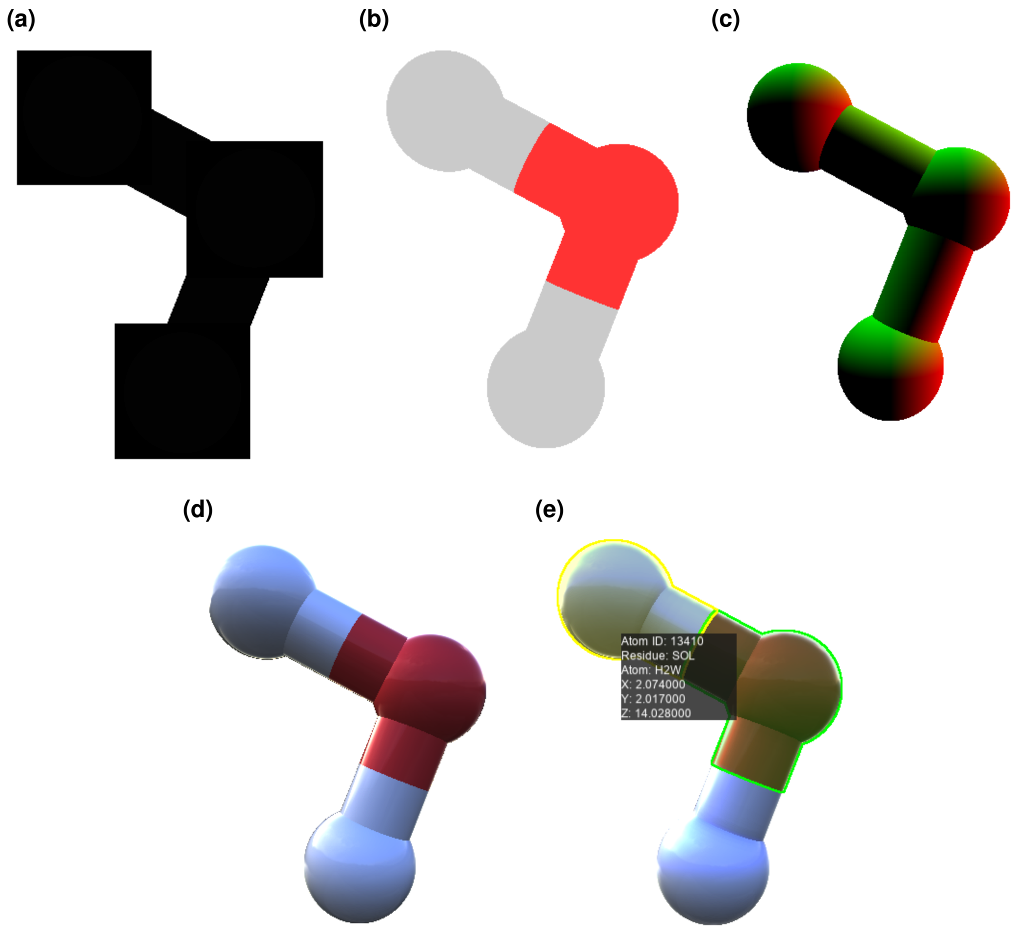


**S3 Fig..** The rendering procedure. (a) Bounding quads are generated using a vertex shader. (b)(c) Surface information channels are generated using ray-tracing in a fragment shader. (d) A Physically-based Rendering (PBR) shader combines the channels into the final image. (e) By utilizing deferred shading, UI overlays and image effects can be added without re-drawing the whole scene, thus improving performance.

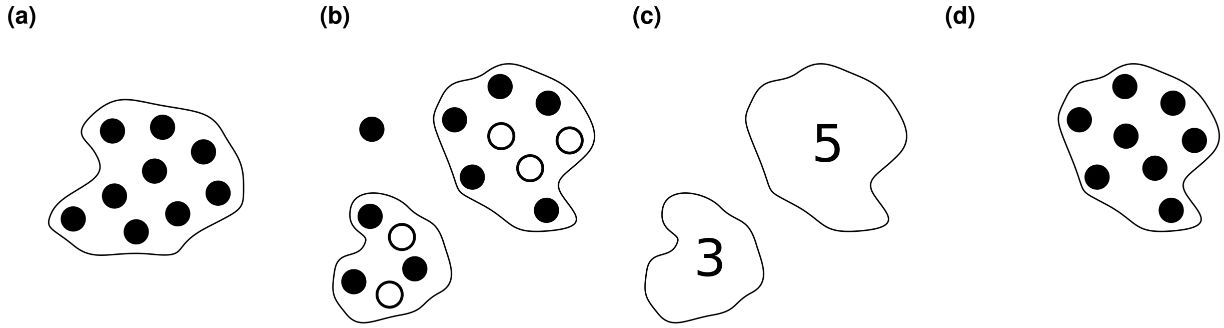


**S4 Fig..** The visual representation of the tracking algorithm. (a) The current frame. (b) The next frame. (c) The number of particles belonging to the previous cluster is counted. (d) The labels are updated for the cluster with the largest count.

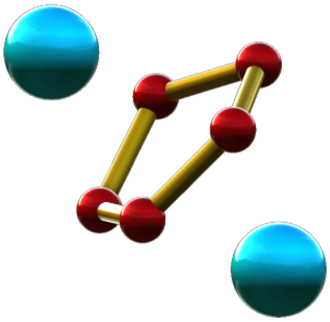

**S5 Fig..** Representation of the mutually coordinated guest order parameter used in the case study on clathrate hydrates. The algorithm is presented by Barnes *et al.*([16] in main text).

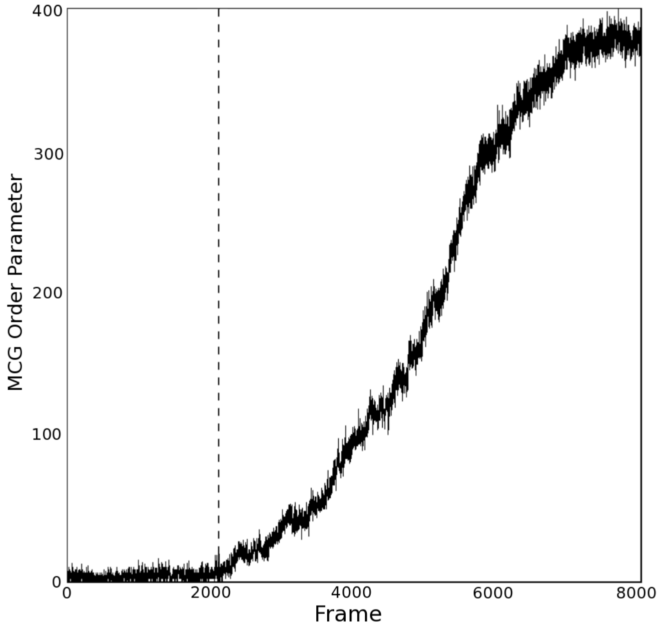


**S6 Fig..** The value of the order parameter across the whole trajectory. From this graph, we can identify the point of hydrate formation at about frame 2000.
